# Supplementary material for: Challenging the Human-in-the-loop in Algorithmic Decision-making
Source: arXiv:2405.10706 source file (2024-08-20)
Supplement: Supplementary file 1 [file appendix.tex]

\section{Space Considerations}

\begin{center}
\begin{tabular}{c|c|c}
  \toprule
    Section & Length & Date Draft \\\midrule
    0. Abstract            & 0.5 pages & \\
    1. Introduction        & 1.5 pages &  \\
    2. Conceptualization   & 1.5 pages &  \\
    3. Philosophical Cons. & 3 pages   & \\
    4. ML Stuff            & 5 pages   &  \\
    5. Related Work        & 1 page    &  \\
    6. Discussion          & 1 page    & \\
    7. Conclusion          & 0.5 pages & \\\midrule
    Total & 13 pages \\
     \bottomrule
\end{tabular}
\end{center}

\section{TODO}

\begin{enumerate}[label=$\square$]
    \item \sebastian{Add confounders independent of the state to the figure?}

    \item \sebastian{Beautify Figure~\ref{fig:framework-human-readble}.}

    \item Experimentally illustrate how the HIL can significantly modify the taking of the algorithms; also ask the other way round: what is the HIL allowed to do without changing the algorithms ranking (Overseeing the overseer)

    \item Constrained optimization problem?
      Weighted combination of values + constraints on values => What can HIL do and why should HIL take action? Model is wrong for the purpose. Something in the model/pipeline is wrong. HIL has its own agenda. HIL is not well aligned with the goals of the political decision-makers. How many degrees of freedom can HIL have to keep the order of algorithms. How can this serve as providing insights into how to limit power? HIL has access to different features.

    \item Understanding what a human can 
    
    \item Explanations for contrasting algorithms
    
    \item Certificates for explanations (e.g., they are not adversarial, one can obtain all information, et.c)
    
    \item Two possible ways for democracy: (i) spell out values and build model which satisfies those (subject to political backdoors); (ii) inspect models
    
    \item Voters can assess different things if given explanation $E_1, E_2,$ or $E_3$, e.g., $E_2$ only let's one check for appropriate treatment assignment, while $E_3$ gives an idea of whether society is moving in the right direction.

    \item Using only a single type of explanation can be insufficient or ineffective for informing the people.
\end{enumerate}

\section{Other stuff}

\subsection{The Role of the Human-in-the-loop}

But what is the actual role of the human-in-the-loop?
Most contemporary research papers don't specify the precise role of this important person not in detail or study it in abstract form, e.g., whether a human-in-the-loop would improve trust in ADM which likely comes with the implicit assumption that the HIL performs ethical decisions in cases in which ADM might not.
But to understand the information needs of the political decision-makers and the factual decision-makers better, we need a more precise characterization.
We can imagine the following objectives a HIL might pursue.
\begin{itemize}
    \item Correcting ADM's mistakes. But what is to be considered a mistake?
      \begin{itemize}
          \item Decisions which would violate constraints imposed by law but were unnoticed before.
          \item Decisions which are not in line with the political decision-makers decisions.
      \end{itemize}
      
    \item Making more-pronounced case-by-case decisions than the ADM.
      This is however might be at odds with the intent of the political decision-makers.
      
    \item Making decisions which are better than the algorithm's decision with respect to the political decision-makers intent to compensate for modelling errors or not accounting for latent confounding factors.
      
    \item A personal agenda not in line with the political decision-makers.
\end{itemize}
The possible objectives mentioned above should be dealt with very differently.
If the HIL corrects the ADM's mistakes frequently, the used algorithm should be adjusted.
Similarly, in cases in which the HIL can make better decisions as compared to the model.
However, the other cases deserve special attention as they have direct consequences regarding the information needs and the types of explanations that should be considered.

\section{Other Stuff 2}

To understand how changes in the anticipated assignment policy influence the goal of the political decision makers, we consider the statistics of the joint distribution of $Y,X$, similarly as in~\cite{kasy2021fairness}.

\begin{itemize}
  \item Value estimation problem
    \begin{itemize}
      \item $E_1$ and $E_2$ are insufficient as the impact is only quantified through $P(S_{t+1}^i | S_t^i, T_t^i)$.
    \end{itemize}
  \item Ranking problem
  \item Effective explanations $\leftrightarrow$ machine teaching
  \item Adversarial explanations
  \item Realizabiltiy of explanations
  \item Feasibility of desired value changes?
\end{itemize}

Considered explanations:
\begin{itemize}
  \item Samples
  \item Counterfactuals
  \item Lime
\end{itemize}

\subsection{Value Estimation}

A central challenge is the estimation of conditional expectations of the states of the individuals.
If the explanations enable the people to perform such estimations, they can verify whether an ADM helps realize their values, e.g., whether subpopulations are treated similarly (e.g., no discrimination because of gender) or whether the change of properties of the subpopulation is going in the desired direction (e.g., subpopulations are treated more fairly than before).

\paragraph{Warm-up: Perfect knowledge about everything but $P_t^i$.}
As a first step, we can consider the case in which all aspects of the sequential-decision making problem except for $P_t^i$ are known by the voters. 
In this setting, except for trivial cases, voters must be able to obtain sufficient information about $P_t^i$ to estimate the expectations.

A key challenge for the people is to assess conditional expectations based on explanations for the different possible algorithms.
\begin{definition}[Value estimation problem]
  Given explanations $E_1$, $E_2$, or $E_3$, estimate conditional expectations regarding $S_{t+1}^i$.
\end{definition}
Intuitively, explanations of type $E_1$ and $E_2$ are insufficient for solving the value estimation problem in general as no information is provided regarding how predictions influence treatments ($E_1$) or no information is provided on how treatments affect the population and if people have incorrect priors regarding this influence they might draw incorrect conclusions (make incorrect value estimates).
\sebastian{How to think about prior knowledge/prior assumptions of the people? How can we formalize it?}
\begin{theorem}
  Explanations of type $E_1$ and $E_2$ are in general insufficient to perform value estimations.
  Explanations of type $E_3$ can be sufficient but might require exponentially many samples.
\end{theorem}
\begin{proof}
  Standard machine learning theory.
\end{proof}

\begin{itemize}
    \item Requirements for a voter to rank the algorithms?
    \item 
\end{itemize}

\begin{theorem}
  Even if a voter knows $P(S_t)$, $P(S_{t+1} | T_t)$ but only observers a finite number of samples and the corresponding evaluation from $\alg_i$, this can be insufficient to decide on the algorithm best aligned with the voter's values.
\end{theorem}
\begin{proof}
  Sketch: (1) Labeled data $\Leftrightarrow$ explanations of the algorithms decisions. (2) Approximation of the algorithms decisions depends on the chosen approximation family and the number of samples. (3) Amount of available information might be insufficient to rank algorithms according to values.
\end{proof}

\paragraph{Others.}

\begin{itemize}
    \item Adversarial explanations wrt to humans understanding.
    \item How much information does an explanation provide?
\end{itemize}

\sebastian{@Eugenia: Please go ahead.}

\subsection{The Role of the Human-in-the-loop}

But what is the actual role of the human-in-the-loop?
Most contemporary research papers don't specify the precise role of this important person not in detail or study it in abstract form, e.g., whether a human-in-the-loop would improve trust in ADM which likely comes with the implicit assumption that the HIL performs ethical decisions in cases in which ADM might not.
But to understand the information needs of the political decision-makers and the factual decision-makers better, we need a more precise characterization.
We can imagine the following objectives a HIL might pursue.
\begin{itemize}
    \item Correcting ADM's mistakes. But what is to be considered a mistake?
      \begin{itemize}
          \item Decisions which would violate constraints imposed by law but were unnoticed before.
          \item Decisions which are not in line with the political decision-makers decisions.
      \end{itemize}
      
    \item Making more-pronounced case-by-case decisions than the ADM.
      This is however might be at odds with the intent of the political decision-makers.
      
    \item Making decisions which are better than the algorithm's decision with respect to the political decision-makers intent to compensate for modelling errors or not accounting for latent confounding factors.
      
    \item A personal agenda not in line with the political decision-makers.
\end{itemize}
The possible objectives mentioned above should be dealt with very differently.
If the HIL corrects the ADM's mistakes frequently, the used algorithm should be adjusted.
Similarly, in cases in which the HIL can make better decisions as compared to the model.
However, the other cases deserve special attention as they have direct consequences regarding the information needs and the types of explanations that should be considered.
